# Supplementary material for: Enhanced magnetic dichroism in darkfield UV photoemission electron microscopy
Source: arXiv:2409.04771 source file (2025-05-15)
Supplement: Supplementary file 1 [file supplement.pdf]

# Magnetic dichroism in darkfield UV photoemission electron microscopy

## — Supplemental Material —

Maximilian Paleschke,<sup>1</sup> David Huber,<sup>1</sup> Friederike Wühl,<sup>1</sup> Cheng-Tien  
Chiang,<sup>2</sup> Frank O. Schumann,<sup>3</sup> Jürgen Henk,<sup>1</sup> and Wolf Widdra<sup>1</sup>

<sup>1</sup>*Institute of Physics, Martin Luther University  
Halle-Wittenberg, D-06099 Halle (Saale), Germany*

<sup>2</sup>*Institute of Atomic and Molecular Sciences, Academia Sinica, Taipei, Taiwan*

<sup>3</sup>*Max-Planck-Institut für Mikrostrukturphysik, 06120 Halle, Germany*

## ELECTRONIC-STRUCTURE AND PHOTOEMISSION CALCULATIONS

For the calculations of the electronic structure and the photoemission intensities we used our computer program package OMNI, which is based on the spin-polarized relativistic layer Korringa-Kohn-Rostoker method (KKR; a brief introduction can be found in Ref. 1). Solving the Dirac equation for a magnetic material, exchange splitting and spin-orbit coupling are treated on equal footing. OMNI has proven its quality in a number of publications, see for example Ref. 3 and references therein.

The sample is taken as semi-infinite Fe(100), for which the muffin-tin potentials of the first seven layers deviate from that of bulk layers. For the image-potential barrier we take a smooth shape described in Ref. 4.

Self-consistent electronic-structure calculations have been performed using the local spin-density approximation for the exchange-correlation functional in density-functional theory. For solving the single-site scattering problem, the layer-KKR method uses an expansion of the scattering solutions with respect to angular momentum, in this work up to  $l_{\max} = 3$ . The potentials of the seven outermost layers of the semi-infinite system differ from that of the remainder (bulk). The interlayer scattering relies on a plane-wave expansion, here with at least 45 beams. The calculated bulk and the surface electronic structures as well as the layer-resolved magnetic moments agree with those computed and published elsewhere.

The results of the electronic-structure calculations serve as basis for the spin- and angle-resolved photoemission calculations, for which the same potentials as for the electronic-structure calculations are used. The spin-polarized photocurrent is calculated within the one-step model of photoemission, taking a time-reversed LEED state as final state. Photoelectrons excited within the topmost 50 layers are considered in order to obtain converged intensities and spin polarizations. The calculated spin-density matrix of the photoelectron allows to derive all components of the photoelectron's spin polarization vector.

In order to mimic many-particle effects, we use an energy-dependent self-energy  $\Sigma(E)$  whose real part shifts electronic states in energy and its imaginary part broadens the photoemission spectra. This energy dependence is modelled by smooth functions while the true self-energy is more complicated and, on top of this, depends on the wave vector  $\mathbf{k}_{\parallel}$  (see for example Ref. 3). This means that one can expect deviations between experimental and theoretical data taken at constant binding energy (confer Figs. 2 and 3 of the main text).

TABLE I. Effect of symmetry operations on the photoelectron wavevector  $\mathbf{k}_{\parallel} = (k_x, k_y)$ , the helicity of the incident light  $\sigma_{\pm}$ , and the in-plane magnetization  $\mathbf{M} = (M_x, M_y)$ . For details see text.

| operation      | wavevector helicity magnetization |        |                |        |       |
|----------------|-----------------------------------|--------|----------------|--------|-------|
| $\hat{1}$      | $k_x$                             | $k_y$  | $\sigma_{\pm}$ | $M_x$  | $M_y$ |
| $\hat{m}_{xz}$ | $k_x$                             | $-k_y$ | $\sigma_{\mp}$ | $-M_x$ | $M_y$ |

## SYMMETRY ANALYSIS

The point group of a nonmagnetic bcc(100) surface is  $C_{4v}$  ( $4mm$ ), which in the case of photoemission from ferromagnetic Fe is reduced to  $C_s$  ( $m$ ), if the light impinges within a mirror plane of the lattice (here: the  $xz$ -plane; confer Fig. 1 of the main text). The two symmetry operations are thus the identity  $\hat{1}$  and the reflection  $\hat{m}_{xz}$  at the  $xz$ -plane. The effect of these operations on the photoelectron's wavevector  $\mathbf{k}_{\parallel} = (k_x, k_y)$ , on the helicity  $\sigma_{\pm}$  of the circular polarized light, and on the in-plane magnetization  $\mathbf{M} = (M_x, M_y)$  is given in Table I.

Table I allows to derive relations between photoemission intensities  $I(k_x, k_y; \sigma_{\pm}; M_x, M_y)$  for equivalent setups. For example, photoemission from a ferromagnetic domain with magnetization along the  $x$ -axis ( $M_y = 0$ ) yields

$$I(k_x, k_y; \sigma_+; M_x, 0) = I(k_x, -k_y; \sigma_-; -M_x, 0). \quad (1)$$

If  $k_y = 0$  (detection in the  $xz$ -plane) one obtains the established relation that the intensity is not changed if both magnetization and helicity are reversed. Likewise, the relation

$$I(k_x, k_y; \sigma_+; 0, M_y) = I(k_x, -k_y; \sigma_-; 0, M_y) \quad (2)$$

tells that for a domain with magnetization along the  $y$ -axis reversing both the azimuth ( $k_y \rightarrow -k_y$ ) and the helicity yield the same intensity. Moreover, generalizing these examples allows to derive the symmetry of the patterns shown in Figs. 2 and 3 of the main text.

The above considerations yield relations between intensities for photoelectrons emitted with opposite azimuths, that is with  $\mathbf{k}_{\parallel} = (k_x, k_y)$  and  $\mathbf{k}_{\parallel} = (k_x, -k_y)$ . Since photoelectrons from both azimuths are detected in a PEEM, the exchange asymmetry can in general be increased if only photoelectrons of one chosen azimuth  $\mathbf{k}_{\parallel}$  are considered; the others are ignored by placing an aperture within the PEEM's beam path.

For a fixed  $\mathbf{k}_{\parallel}$  we define asymmetries that disentangle the contrast mechanisms: light polarization ( $A_{\text{pol}}$ ) and magnetization orientation ( $A_{\text{ex}}$ ). With the four intensities  $I(\mathbf{k}_{\parallel}, \sigma_{\pm}, \pm M)$ , in the following shortened as  $I_{\pm\pm}$ , we define the total intensity

$$I \equiv I_{++} + I_{+-} + I_{-+} + I_{--} \quad (3)$$

and the respective asymmetries

$$A_{\text{pol}} \equiv [(I_{++} + I_{+-}) - (I_{-+} + I_{--})] / I, \quad (4a)$$

$$A_{\text{ex}} \equiv [(I_{++} + I_{--}) - (I_{+-} + I_{-+})] / I. \quad (4b)$$

A third asymmetry,

$$A_{\text{soc}} \equiv [(I_{++} + I_{-+}) - (I_{+-} + I_{--})] / I, \quad (5)$$

quantifies the spin polarization produced by optical orientation, aka Fano effect, which requires spin-orbit coupling (SOC).

- 
- [1] J. Henk, Theory of low-energy diffraction and photoelectron spectroscopy from ultra-thin films, in [2], Chap. 10, p. 479.
  - [2] H. S. Nalwa, ed., *Handbook of Thin Film Materials* (Academic Press, San Diego, 2002).
  - [3] C. Tusche, M. Ellguth, V. Feyer, A. Krasnyuk, C. Wiemann, J. Henk, C. M. Schneider, and J. Kirschner, Nonlocal electron correlations in an itinerant ferromagnet, [Nature Communications](#) **9**, 3727 (2018).
  - [4] J. Henk, W. Schattke, H. Cartensen, R. Manzke, and M. Skibowski, Surface-barrier and polarization effects in the photoemission from GaAs(110), [Physical Review B](#) **47**, 2251 (1993).
